# Supplementary material for: Towards Understanding Limitations of Pixel Discretization Against Adversarial Attacks
Source: arXiv:1805.07816 source file (2019-10-03)
Supplement: Supplementary file 1 [file appendix.tex]

\section{Proofs for Idealized Conditions}
\label{app:ideal}

% \begin{center}
% \begin{tabular}{| c | c | c | c |}
% \hline
%  Number of Codes & accuracy (pre-trained) & robustness(pre-trained) \\ \hline
%  10(r=64) & 53.90\% & 4.30\% \\ \hline
%  50(r=48) & 77.10\% &  2.60\% \\ \hline
%  100(r=16) & 88.40\% &  2.00\% \\ \hline
%  200(r=16) & 89.50\% & 2.50\% \\ \hline
%  300(r=16) & 89.30\% & 2.50\% \\ \hline
%  $256^3$ (all) & 94.50\% & 2.60\% \\ \hline
% \end{tabular}
% \end{center}

% \subsection{Effect of Random Noise}
% \yingyu{show the tradeoff between natural accuracy and robustness; show that exploiting data properties is more effective than adding random noise without using data properties}

%%% Local Variables:
%%% mode: latex
%%% TeX-master: "make"
%%% End:
